# Supplementary material for: Electrically Tunable Magnonic Bound States in the Continuum
Source: arXiv:2502.18260 source file (2025-02-25)
Supplement: Supplementary file 1 [file Supplemental_Material.pdf]

# Supplemental Material: Electrically Tunable Magnonic Bound States in the Continuum

Xi-guang Wang[1], Guang-hua Guo[1], Jamal Berakdar[2], Hui Jing[3*]

[1] *School of Physics, Central South University, Changsha 410083, China*

[2] *Institut für Physik, Martin-Luther Universität Halle-Wittenberg, 06099 Halle/Saale, Germany*

[3] *Key Laboratory of Low-Dimensional Quantum Structures and Quantum Control of Ministry of Education, Department of Physics and Synergetic Innovation Center for Quantum Effects and Applications, Hunan Normal University, Changsha 410081, China*

[*] *email: jinghui73@gmail.com*

(Dated: December 8, 2024)

## I. TECHNICAL DETAILS OF THE NUMERICAL SIMULATIONS

The Landau-Lifshitz-Gilbert (LLG) equation is numerically solved using a fifth-order Runge-Kutta scheme with a fixed time step of 0.1 ps. Two coupled waveguides WG1 and WG2 are discretized with a cell size of 2 nm along the $x$ axis. In the numerical simulation, the magnetization is renormalized to saturation magnetization $M_{\mathrm{s}}$ before evaluating the magnetic effective fields at each step. The accuracy of our code has been validated against several standard problems, showing excellent agreement with results obtained from the OOMMF. In the simulations, we first let the magnetization relax to a stationary state ($+y$ direction in WG1 and $-y$ direction in WG2), and then add the magnon excitation to the coupled waveguides via microwave fields. The magnon amplitude is determined from the oscillation amplitudes of the $m_{\mathrm{x}}(x,t)$ and $m_{\mathrm{z}}(x,t)$ components of the magnetization.

## II. DISCUSSION ON THE EP

In this section, we provide more details about the exceptional point (EP) in the antiferromagnetically coupled waveguides with intrinsic loss and additional loss. Under small damping $\alpha \to 0$, from the Hamiltonian Eq. (2) in the main text, we obtain the eigenfrequencies of the two magnon modes as,

$$\omega_{\pm} = \sqrt{\omega_0^2 - \omega_{\mathrm{z}}^2 - \kappa^2 - \frac{\omega_{\mathrm{c}}^2}{4} \mp \sqrt{(4\kappa^2\omega_{\mathrm{z}}^2 - \omega_{\mathrm{c}}^2(\omega_0^2 - \omega_{\mathrm{z}}^2)}} - \frac{i\omega_{\mathrm{c}}}{2}. \tag{S1}$$

For $\omega_{\mathrm{c}} < \frac{2\kappa\omega_{\mathrm{z}}}{\sqrt{\omega_0^2-\omega_{\mathrm{z}}^2}}$, the real parts of $\omega_{\pm}$ are always separate, and the imaginary parts $-\frac{i\omega_{\mathrm{c}}}{2}$ are identical and simultaneously increase with $\omega_{\mathrm{c}}$. At $\omega_{\mathrm{c}} = \frac{2\kappa\omega_{\mathrm{z}}}{\sqrt{\omega_0^2-\omega_{\mathrm{z}}^2}}$, $\omega_{\pm}$ coalesce at the same value, which is the hallmark of the non-Hermitian degeneracy or the EP. Above the EP, the real parts of $\omega_{\pm}$ have the same value, and the two imaginary parts are separated. Numerical calculations based on Eq. (S1) validate these features, as shown in Figs. S1(a-b).

We note that $\alpha = 0.01$ is used in the main article. For YIG, depending on the YIG-film fabrication method, $\alpha$ can be three orders smaller. When we consider a small damping $\alpha = 0.0001$ (Figs. S1(c-d)), the small damping induced difference in the EP is negligible. Larger $\alpha = 0.01$ causes a small gap at the EP region (Figs. S1(e-f)), making the EP somewhat unclear. However, we can still identify the features above EP, i.e., more separated imaginary parts and almost collapsed real parts. Besides, around the additional loss induced EP, the imaginary parts of $\omega_{\pm}$ are always negative, indicating that passing through the EP

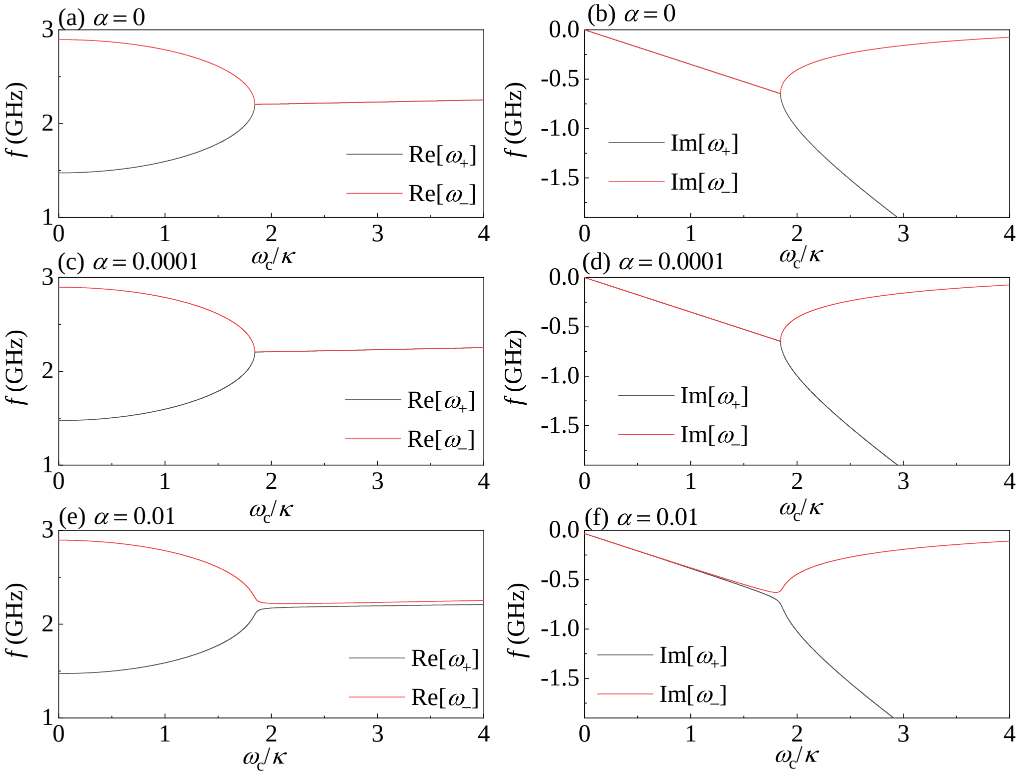


FIG. S1. For (a-b) $\alpha = 0$, (c-d) $\alpha = 0.0001$ and (e-f) $\alpha = 0.01$, the real and imaginary parts of magnon eigenfrequencies as the WG1 electric current term $\omega_c/\kappa$ varies. Here, $k_x = 0$.

does not induce magnon amplification or magnetization flipping. This suggests that the addition loss induced EP we found is different from the EP resulting from coupled gain and loss, where the ground state may change and nonlinear oscillation may arise.[1, 2]

## III. DISCUSSION ON THE ENHANCED LOSS AND BIC

First, we provide more details about the spin orbit torque (SOT) induced enhanced loss in WG1. It has been well documented that, depending on the direction of the electric current, the SOT can either enhance or reduce the magnon loss in the attached waveguide. To demonstrate this feature, we remove the interlayer coupling $\kappa$ and assume a single waveguide WG1 with SOT $\mathbf{T}_1 = \gamma c_J \mathbf{m}_1 \times \mathbf{y} \times \mathbf{m}_1$. The Hamiltonian (Eq. (2)) in the main text becomes a $2 \times 2$ Hamiltonian $\hat{H}_s$,

$$\hat{H}_s = \begin{pmatrix} \omega_0^- - i\omega_J^- & -\omega_z^- \\ \omega_z^+ & -\omega_0^+ - i\omega_J^+ \end{pmatrix} \tag{S2}$$

and the single eigenfrequency is obtained as,

$$\omega_{\rm s} = \sqrt{(\omega_0 - \alpha\omega_{\rm c})^2 - (1+\alpha^2)\omega_{\rm z}^2} - i(\alpha\omega_0 + \omega_{\rm c}). \tag{S3}$$

The equation clearly proves that a positive $\omega_{\rm c}$ increases the imaginary part of the magnon mode of WG1, i.e. additional magnon loss, and the $\alpha\omega_0$ term represents the intrinsic loss from Gilbert damping, as demonstrated by the numerical results in Fig. S2. Reversing the direction of the electric current ($\omega_{\rm c} < 0$), the SOT turns into an antidamping torque and plays the role of gain.

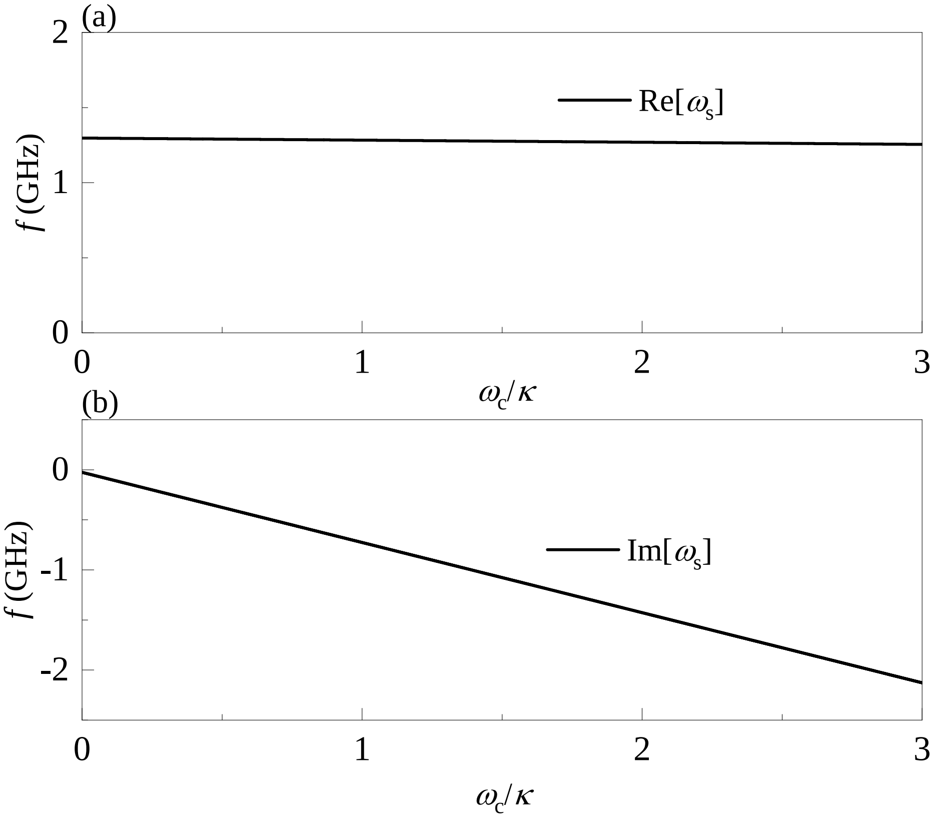


FIG. S2. For $\alpha = 0.01$ and $k_{\rm x} = 0$ nm$^{-1}$, the real and imaginary parts of magnon eigenfrequency as the single WG1 electric current term $\omega_{\rm c}$ varies. Here, $\omega_{\rm c}$ is rescaled by the term $\kappa$ of the coupled waveguides.

For the coupled WG1 and WG2 in the main article, it is the additional loss ($\omega_{\rm c} > 0$) that generates the BIC. In the field of BIC research, one key method for generating BIC is typically to tune the parameters in a system with two (or more) resonant structures coupled to the same channel. BICs can be formed between two resonant structures by adjusting the

frequencies or structure parameters. A Friedrich-Wintgen (FW) BIC can occur by tuning a certain set of structural parameters in the non-Hermitian Hamiltonian of two connected resonant structures,[3–5]

$$\hat{H}_{\rm t} = \begin{pmatrix} \omega_{\rm t1} - ir_1 & \kappa_{\rm t} - i\sqrt{r_1 r_2} \\ \kappa_{\rm t} - i\sqrt{r_1 r_2} & \omega_{\rm t2} - ir_2 \end{pmatrix}. \tag{S4}$$

Here, two coupled resonators have different resonance frequencies $\omega_{\rm t1,t2}$ and different radiation rates $r_{1,2}$. The two resonators are coupled to the same channel via $\kappa_{\rm t}$ term. Without coupling, the two resonators have independent decay rates related to the positive real-valued $r_{1,2}$. Allowing the coupling, and when the FW condition $\kappa_{\rm t}(r_1 - r_2) = \sqrt{r_1 r_2}(\omega_{\rm t1} - \omega_{\rm t2})$ is met, the imaginary part of one eigenvalue becomes 0 (lossless BIC), and the imaginary part of the other eigenvalue $-(r_1 + r_2)$ accounts for all the losses. The FW condition is achieved by tuning the radiation rates $r_{1,2}$ within the positive range, leading to the appearance of a lossless mode by introducing coupled losses without any gain.

The magnonic BIC in the main article shares similar features with the FW BIC: (i) Two separated magnetic layers WG1 and WG2 can be regarded as two different resonators. Without the coupling, the two resonators mode frequencies $\omega_{\rm WG1} = \sqrt{(\omega_0 - \alpha\omega_{\rm c})^2 - (1+\alpha^2)\omega_{\rm z}^2} - i(\alpha\omega_0 + \omega_{\rm c})$ and $\omega_{\rm WG2} = \sqrt{\omega_0^2 - (1+\alpha^2)\omega_{\rm z}^2} - i\alpha\omega_0$, have different radiation rates. The coupling channel between the resonators is provided by the interlayer interaction with coupling-field strength $\kappa$. (ii) By tuning the $\omega_{\rm c}$ term, one eigenvalue turns into a BIC (purely real), and the imaginary part of the other eigenvalue significantly increases (more lossy). For example, at $k_{\rm x} = 0$ and $\omega_{\rm c} = 13.2\kappa$, the resonances in separated WG1 and WG2 have imaginary parts of ${\rm Im}[\frac{\omega_{\rm (WG1,WG2)}}{2\pi}] = (-9.26, -0.03)$ GHz without coupling interaction. Including the coupling, the magnonic BIC ${\rm Im}[\frac{\omega_{(+,-)}}{2\pi}] = (-9.29, 0)$ GHz emerges. Same as for FW BIC, the other $\omega_+$ mode attains all the losses. (iii) The additional loss ($\omega_{\rm c} > 0$) induced BIC is generated by the non-Hermitian effect, which is unrelated to antidamping torque or gain. From these features, as the magnonic Hamiltonian not being a typical FW Hamiltonian, the magnonic BIC can be recognized as an unconventional BIC.

## IV. ENHANCED MAGNON EXCITATION NEAR BIC

To prove the enhanced magnon excitation near the BIC, we apply an out-of-plane external microwave field $h_{\rm z} e^{ik_{\rm x}x - i\omega t}$ along the $z$ direction. Including the microwave field in the LLG

equation, we write $\Psi_{\rm p}^{+} = \sum_{\rm p'} \chi_{\rm pp'}(\omega) h_{\rm z}^{p'}$ with the dynamic magnetic susceptibility being $\chi_{\rm pp'}(\omega)$. Fig. S3 shows how the susceptibility depends on electric current strength $\omega_{\rm c}$, with the case of $k_{\rm x} = 0$ provided for illustration. Exciting magnons of $\omega_{-}$ mode results in a significant increase in magnetic susceptibility $\chi_{\rm pp'}$ at the BIC ($\omega_{\rm c} = 13.2\kappa$). Despite the fact that the $\omega_{+}$ mode does not feature a BIC, a weaker enhancement in magnetic susceptibility is still observed.

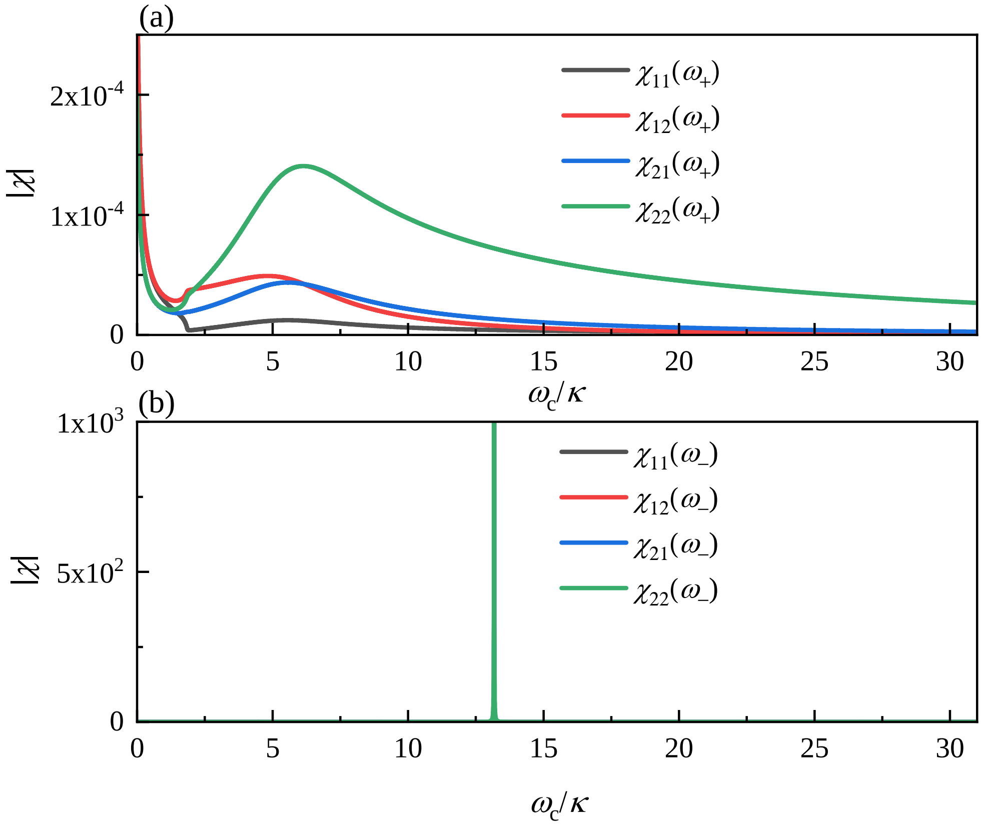


FIG. S3. At $k_{\rm x} = 0$, the susceptibility amplitudes $|\chi|$ as functions of $\omega_{\rm c}$. (a) and (b) correspond to the magnon modes of $\omega_{+}$ and $\omega_{-}$ respectively.

## V. CONTROL OF MAGNONS VIA ELECTRIC CURRENT PULSE

For the structure of Fig. 4 in the main article, it is not required to terminate the current exactly when the magnons leave the coupling region. In fact, it is at the moment of current termination, that the magnons can transition to a non-BIC mode and leave the coupling region. For example, if we terminate the current at $t = 45$ ns, magnons begin propagating

to the right at the same moment, as demonstrated by Fig. S4.

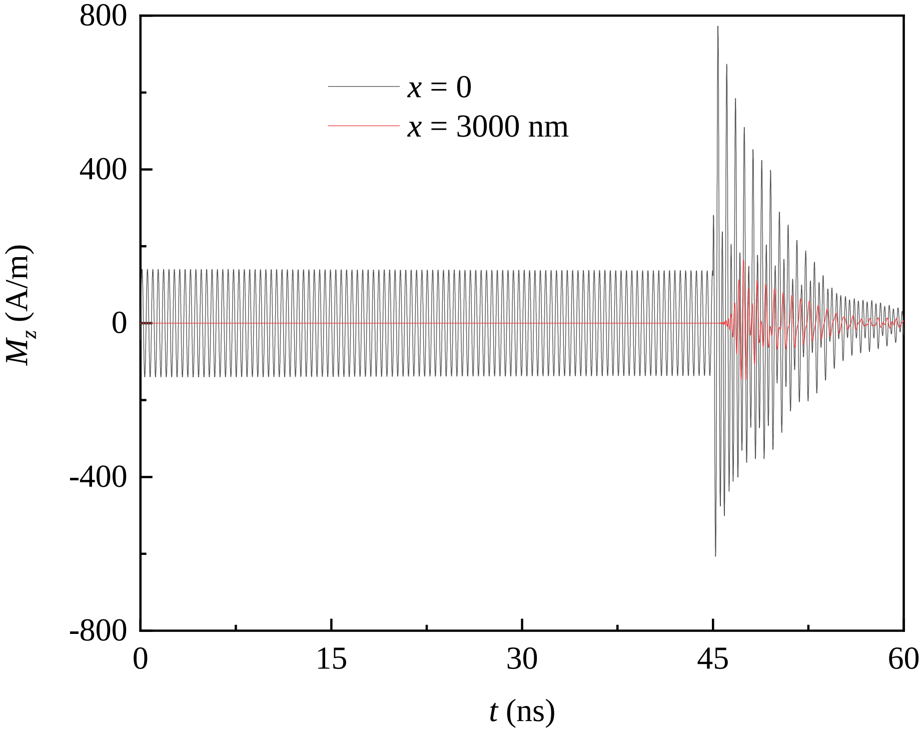


FIG. S4. Adopting the structure of Fig. 4 in the main article, time-resolved oscillations of $M_z$ at the $x = 0$ and $x = 3000$ nm in WG1. Here, the electric current with $\omega_c = 13.2\kappa$ is injected over $0 < t < 45$ ns.

## VI. DISCUSSION ON THE MULTIPLE BICS

In the main article, when the magnetic parameters place the system above the single BIC state, two BICs appear. Here, we present a more detailed discussion of this phenomenon. As demonstrated by Figs. S5(a-b), the imaginary part of one magnon mode becoming zero when $\omega_c = 1.2\kappa$, indicating a lossless mode, i.e. magnonic BIC. Above this specific BIC ($\omega_c = 1.2\kappa$), the imaginary component of the magnon mode turns positive, representing a time-amplifying magnon mode. Subsequently, the imaginary component of the magnon mode descends back to zero, leading to the other relatively higher BIC ($\omega_c = 38.3\kappa$). Upon further increasing the current, i.e. increasing $\omega_c$, the imaginary part of the magnon mode

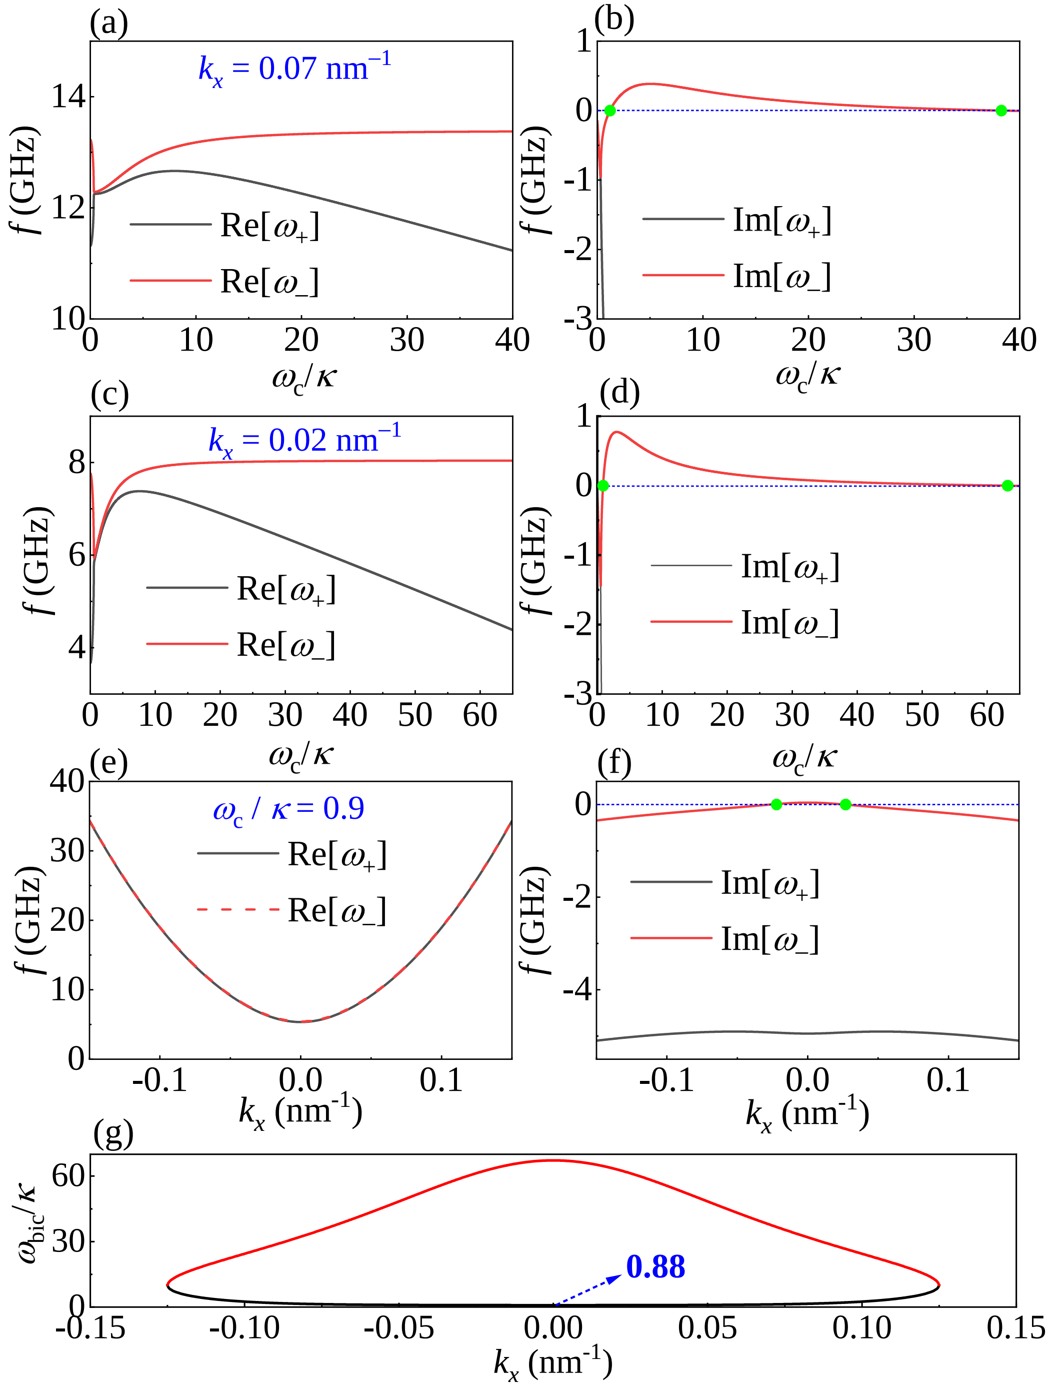


FIG. S5. For (a-b) $k_x = 0.07\text{nm}^{-1}$ and (c-d) $k_x = 0.02\text{nm}^{-1}$ with $J_{AF} = 1.3 \times 10^{-4}$ J/m$^2$, the real and imaginary parts of the magnon eigenfrequencies as the WG1 electric current term $\omega_c/\kappa$ varies where $\omega_c$ ($\kappa$) is linearly proportional to the current density (interlayer WGs coupling). (e-f) With charge current corresponding to $\omega_c = 0.9\kappa$, real and imaginary parts of two magnon eigenfrequencies as functions of the wave vector $k_x$. (g) Values of the critical current $\omega_{BIC}$ of magnon BIC as a function of $k_x$, which is calculated from Eq. (S5). The green points signal the BIC.

turns negative once again. The $\omega_c$ values at the two BIC points change with the variation of the magnon wave vector $k_x$. The comparison of Figs. S5(a-d) demonstrates that different wave vectors $k_x$ result in distinct BICs. This characteristic is also shown in the changes of the magnon mode eigenvalue with $k_x$. As an example, when $\omega_c = 0.9\kappa$ in Figs. S5(e-f), the BICs exclusively emerge at particular wave vectors ($k_x = \pm 0.026\mathrm{nm}^{-1}$). In the interval ($-0.026\mathrm{nm}^{-1} < k_x < 0.026\mathrm{nm}^{-1}$), the magnon mode exhibits a positive imaginary component, in contrast to other $k_x$ regions where the magnon mode's imaginary component remains negative.

Utilizing the condition of zero dissipation, we extract the current values at two BICs,

$$\begin{aligned} \omega_{\mathrm{BIC}}^{\pm} =& \frac{2\kappa^2 + \frac{(1\pm\sqrt{3}i)(\kappa^4-12\alpha^2\omega_0^2\omega_1^2)}{\omega_2^2} + (1\mp\sqrt{3}i)\omega_2^2}{6\alpha\omega_0}, \\ \text{with } \omega_1^2 =& \omega_0^2 - \kappa^2 - \omega_z^2, \\ \omega_2^2 =& [-\omega_3^6 + \frac{1}{2}\sqrt{-4(\kappa^4 - 12\alpha^2\omega_0^2\omega_1^2)^3 + 4\omega_3^{12}}]^{1/3}, \\ \omega_3^6 =& \kappa^6 - 54\alpha^4\omega_0^4(\omega_0^2 - \omega_z^2) + 18\alpha^2\kappa^2\omega^2(\omega_z^2 - \omega_1^2). \end{aligned} \tag{S5}$$

Here, $\omega_{\mathrm{BIC}}^{+}$ and $\omega_{\mathrm{BIC}}^{-}$ represent BICs that exist on the larger and smaller current values respectively. At the BIC condition, the lossless mode only has the real component,

$$\omega = \frac{\sqrt{(1+\alpha^2)[\alpha\omega_c^2\omega_0 + (2\alpha\omega_0 + \omega_c)\omega_1^2]}}{\sqrt{\omega_c + 2\alpha\omega_0}}. \tag{S6}$$

Eq. (S5) can well describe the characteristics of the BICs. From the numerical calculation in Fig. S5(g), it is evident that BIC currents are symmetric for both positive and negative $k_x$. At $k_x = 0$, the smallest ($\omega_{\mathrm{BIC}}^{-} = 0.88\kappa$) and largest ($\omega_{\mathrm{BIC}}^{+} = 67.2\kappa$) currents for BIC exist simultaneously. With the increase in $k_x$, the smaller BIC ($\omega_{\mathrm{BIC}}^{-}$) gradually increases, while the larger BIC ($\omega_{\mathrm{BIC}}^{+}$) progressively decreases. Of significant note is the coincidence of $\omega_{\mathrm{BIC}}^{-}$ and $\omega_{\mathrm{BIC}}^{+}$ when $k_x = \pm 0.125\mathrm{nm}^{-1}$. Afterward, when $|k_x| > 0.125\mathrm{nm}^{-1}$, it is impossible to induce the BIC, regardless of the current magnitude.

Contrary to the typical systems known for exhibiting BIC, our analysis of the anti-ferromagnetically coupled waveguides has revealed two distinct BICs. To understand the fundamental causes behind this phenomenon, we discuss it in the context of the Hamiltonian Eq. (S4) of a typical system. It is well documented that, when the criteria for the Friedrich–Wintgen condition $\kappa_t(r_1 - r_2) = \sqrt{r_1 r_2}(\omega_{t1} - \omega_{t2})$ are met, one eigenmode undergoes a transformation into a non-dissipative form, thus emerging as a BIC mode. For real

numbers $\omega_{t1,t2}$, $r_{1,2}$ and $\kappa_t$, precise modulation of the dissipation rate $r_1$ enables the precise tuning of the system to the BIC, as demonstrated by Fig. S6.

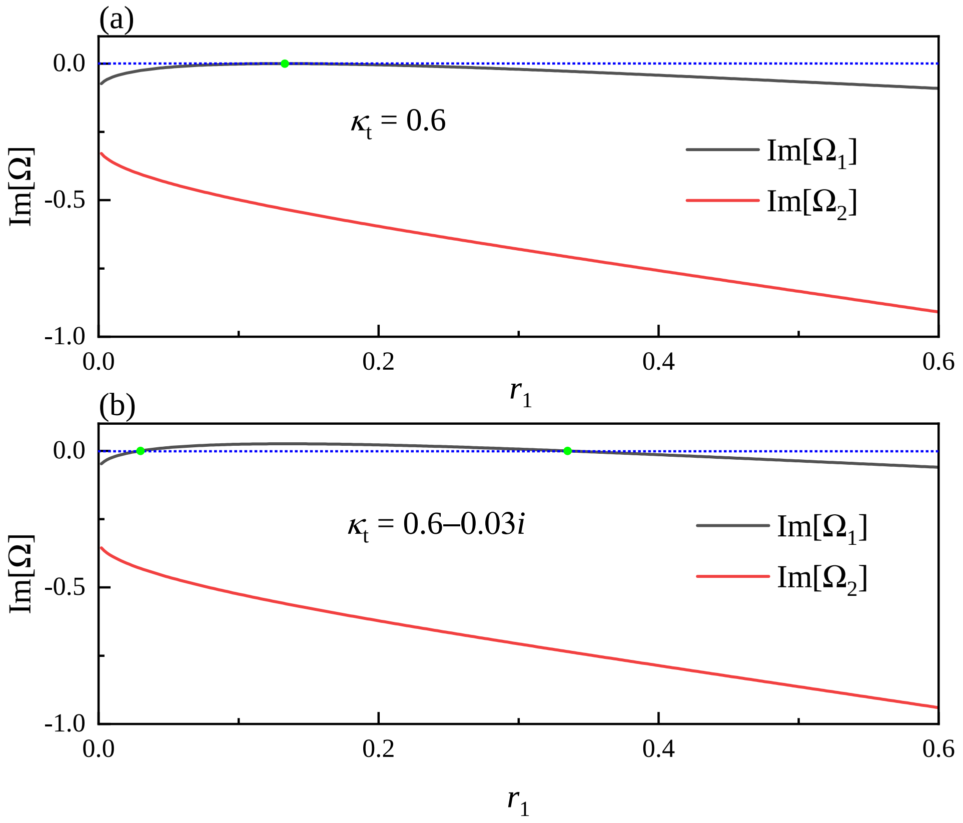


FIG. S6. With the parameters $\omega_{t1} = 1$, $\omega_{t2} = 1.7$, $r_2 = 0.4$, the $r_1$ dependent imaginary parts of the two eigenmodes. Here, we employs a real value $\kappa_t = 0.6$ in (a) and a complex value $\kappa_t = 0.6 - 0.03i$ in (b).

We find that the application of a complex coupling constant $\kappa$ enables the formation of two BICs, as evidenced in Fig. S6. Between the two BICs, the imaginary part of the intrinsic mode evolves from a negative to a positive value, signaling an amplified mode, which is consistent with the observations detailed in the main article. The main article attributes the imaginary component of the coupling constant, which incorporates dissipation, to the influence of the Gilbert damping constant. This qualitatively provides a critical mechanism for understanding multi BICs and the associated amplified mode with positive imaginary part. The presence of two BICs with positive imaginary components has also been observed in cavity magnon-polaritons [6].

## VII. INFLUENCE OF EXTERNAL MAGNETIC FIELD

In this section, we explore in depth the influence of an external magnetic field $H_\mathrm{x}$ applied along the $x$ axis, and elaborate on the discussion of the associated analytical procedures. Under $H_\mathrm{x}$, the originally antiparallel $\mathbf{m}_1 = (0, 1, 0)$ and $\mathbf{m}_2 = (0, -1, 0)$ undergo inclinations along the $x$ axis, thereby generating a spin-flop state, i.e., $\mathbf{m}_\mathrm{p} = (m_\mathrm{p,x}, m_\mathrm{p,y}, m_\mathrm{p,z})$. Utilizing the stability conditions $\frac{\partial \mathbf{m}_\mathrm{p}}{\partial t} = 0$, we derive the changes in the stable spin-flop state as the field $H_\mathrm{x}$ varies, as depicted in Fig. S7. In the absence of electric current ($\omega_\mathrm{c} = 0$), $\mathbf{m}_1$ and $\mathbf{m}_2$ exhibit symmetric variations, with a convergence of the $x$ and $z$ components ($m_\mathrm{z} = 0$), as shown in Fig. S7(a). When the SOT is exclusively applied to WG1, the torque drives the asymmetric trends observed in the changes of $\mathbf{m}_1$ and $\mathbf{m}_2$ (Fig. S7(b)).

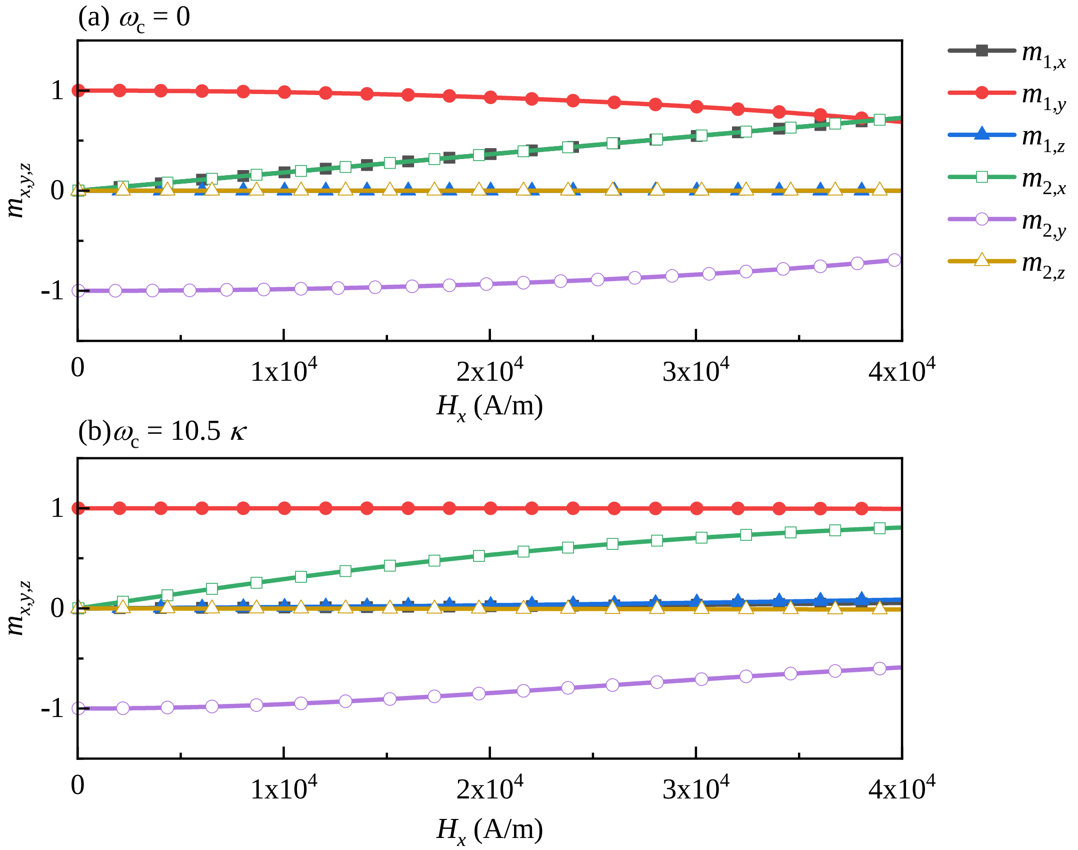


FIG. S7. For (a) $\omega_\mathrm{c} = 0$ and (b) $\omega_\mathrm{c} = 10.5\kappa$, variations in stable magnetization $\mathbf{m}_\mathrm{p}$ with $H_\mathrm{x}$. $p = 1, 2$ enumerate WG1 and WG2.

To consider spin-wave excitations in the spin-flop, we employ spherical coordinates $\theta'_\mathrm{p}$ and $\phi'_\mathrm{p}$, where the stable magnetization $\mathbf{m}_\mathrm{p} = (\sin\theta'_\mathrm{p}\cos\phi'_\mathrm{p}, \sin\theta'_\mathrm{p}\sin\phi'_\mathrm{p}, \cos\theta'_\mathrm{p})$. The spin

flop state is described by $\theta'_{\rm p} = \frac{\pi}{2} - \theta_{\rm p}$ and $\phi'_{1(2)} = +(-)(\frac{\pi}{2} - \phi_{1(2)})$. In the absence of electrical current $\omega_{\rm c} = 0$, there are $\theta_1 = \theta_2$ and $\phi_1 = \phi_2$. The asymmetric torque makes $\theta_1 \neq \theta_2$ and $\phi_1 \neq \phi_2$. Magnons are characterized by small coherent variations around the equilibrium state $\mathbf{m}_{\rm p} + [\delta m_{\theta,{\rm p}}\mathbf{e}_\theta + \delta m_{\phi,{\rm p}}\mathbf{e}_\phi]e^{i(k_{\rm x}x-\omega t)}$. The magnon equation is derived by inserting these expressions into the LLG equation and linearizing. Through $\psi^{\pm}_{\rm r,p} = \delta m_{\theta,{\rm p}} \pm i\delta m_{\phi,{\rm p}}$, the magnon equation can be recast as an eigenvalue problem $\omega\boldsymbol{\psi}_{\rm r} = \hat{H}_{\rm r}\boldsymbol{\psi}_{\mathbf{r}}$ with $\boldsymbol{\psi}_{\rm r} = (\psi^+_{\rm r,1}, \psi^-_{\rm r,1}, \psi^+_{\rm r,2}, \psi^-_{\rm r,2})$. The $4 \times 4$ non-Hermitian Hamiltonian $\hat{H}_{\rm r}$ is,

$$\hat{H}_{\rm r} = \begin{pmatrix} -\omega^{1+}_{\rm r} - i\omega^+_{\rm r,c} & -\omega^{1+}_{\rm r,z} & \kappa^+_1 + i\kappa^+_2 & -\kappa^+_3 - i\kappa^+_4 \\ \omega^{1-}_{\rm r,z} & \omega^{1-}_{\rm r} - i\omega^-_{\rm r,c} & \kappa^-_3 - i\kappa^-_4 & -\kappa^-_1 + i\kappa^-_2 \\ \kappa^+_1 - i\kappa^+_2 & -\kappa^+_3 - i\kappa^+_4 & -\omega^{2+}_{\rm r} & -\omega^{2+}_{\rm r,z} \\ \kappa^-_3 - i\kappa^-_4 & -\kappa^-_1 - i\kappa^-_2 & \omega^{2-}_{\rm r,z} & \omega^{2-}_{\rm r} \end{pmatrix}. \tag{S7}$$

Here, $\omega_{\rm c} = \frac{\gamma c_{\rm J}}{1+\alpha^2}$, $\kappa = \frac{\gamma J_{\rm AF}}{(1+\alpha^2)\mu_0 M_{\rm s} t_{\rm p}}$, $\omega_{\rm z} = \frac{\gamma K_{\rm z}}{(1+\alpha^2)\mu_0 M_{\rm s}}$, $\omega_{\rm y} = \frac{\gamma K_{\rm y}}{(1+\alpha^2)\mu_0 M_{\rm s}}$, $\omega^{1(2)}_{\rm r,ex} = \frac{\gamma}{1+\alpha^2}(\frac{2A_{\rm ex}k_{\rm x}^2}{\mu_0 M_{\rm s}} + \frac{K_{\rm y}(3\cos^2\theta_{1(2)}\cos^2\phi_{1(2)}-1)}{\mu_0 M_{\rm s}} + H_{\rm x}\cos\theta_{1(2)}\sin\phi_{1(2)})$, $\omega^{1(2)}_{\rm r} = \omega^{1(2)}_{\rm r,ex} + \omega_{\rm z}(3\cos^2\theta_{1(2)} - 2) + \kappa[\cos\theta_1\cos\theta_2\cos(\phi_1 + \phi_2) - \sin\theta_1\sin\theta_2]$, $\omega_{\rm r,c} = \omega_{\rm c}\cos\theta_1\cos\phi_1$, $\omega^{1(2)}_{\rm r,z} = \omega_{\rm z}\cos^2\theta_{1(2)} + \omega_{\rm y}[(\cos 2\theta_{1(2)}\cos^2\phi_{1(2)} - 1)/2 - (+)i\sin\theta_{1(2)}\sin 2\phi_{1(2)}]$, $\kappa_1 = \kappa[(\sin\theta_1\sin\theta_2 + 1)\cos(\phi_1 + \phi_2) - \cos\theta_1\cos\theta_2]/2$, $\kappa_2 = \kappa[(\sin\theta_1 + \sin\theta_2)\sin(\phi_1 + \phi_2)]/2$, $\kappa_3 = \kappa[(1 - \sin\theta_1\sin\theta_2)\cos(\phi_1 + \phi_2) + \cos\theta_1\cos\theta_2]/2$, $\kappa_4 = \kappa[(\sin\theta_1 - \sin\theta_2)\sin(\phi_1 + \phi_2)]/2$, $\omega^{1(2)\pm}_{\rm r} = (1 \pm i\alpha)\omega^{1(2)}_{\rm r}$, $\omega^{\pm}_{\rm r,c} = (1 \pm i\alpha)\omega_{\rm r,c}$, $\omega^{1(2)\pm}_{\rm r,z} = (1 \pm i\alpha)\omega^{1(2)}_{\rm r,z}$, and $\kappa^{\pm}_{1,2,3} = (1 \pm i\alpha)\kappa_{1,2,3}$. In the main text, the aforementioned formulation is applied to calculate the characteristics of magnonic BIC within the spin-flop regime.

Here, we provide more discussions on the influences of $H_{\rm x}$ on multiple BICs. Figs. S8(a-b) show that, without electric current ($\omega_{\rm c} = 0$), increasing the magnetic field $H_{\rm x}$ leads to crossing of the real parts of two distinct magnon modes, observed at approximately $H_{\rm x} = 1.1 \times 10^5$A/m. During the process, the imaginary parts of both modes show a slight divergence, consistently maintaining negative values. In Figs. S8(c-d), when the electric current $\omega_{\rm c} = 0.92\kappa$ is injected and the system is above the EP ($\omega_{\rm c} = 0.33\kappa$), the real parts of the two modes coalesce for $H_{\rm x} = 0$, while their imaginary parts are significantly delineated. Notably, increasing the magnetic field to $H_{\rm x} = 1.1 \times 10^5$ A/m, the imaginary component of one mode is reduced to zero, indicating the emergence of a magnon BIC. At $H_{\rm x} = 0$, the BIC necessitates $\omega_{\rm c} = 1.2\kappa$, as depicted in the above Figs. S5(a-b). Furthermore, Figs. S8(e-f) provides the dispersion characteristics for magnon modes at $\omega_{\rm c} = 0.9\kappa$ and $H_{\rm x} = 1.1 \times 10^5$ A/m. Compared to Figs. S5(e-f), there is a notable increase in $k_{\rm x}$ associated with the BIC,

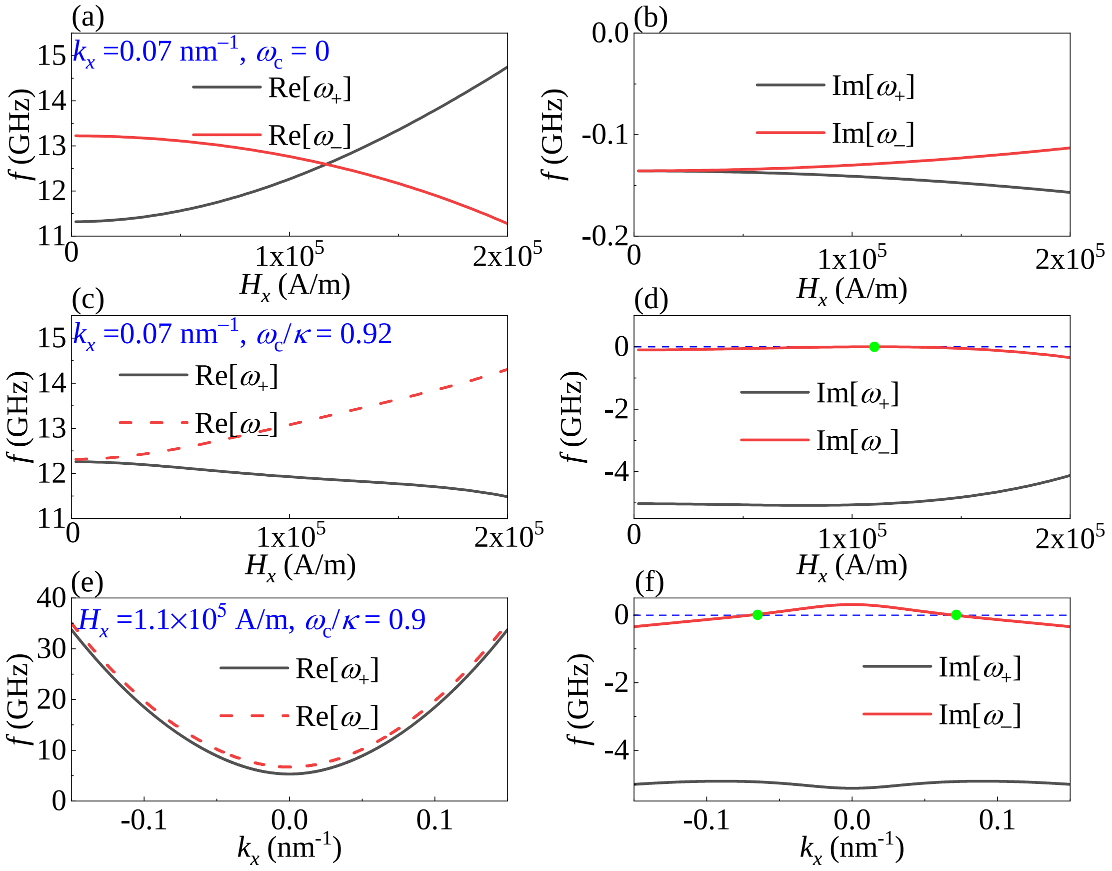


FIG. S8. For (a-b) $\omega_c = 0$ and (c-d) $\omega_c = 0.92\kappa$ with $J_{AF} = 1.3\times10^{-4}$ J/m$^2$, the external magnetic field $H_x$ dependent real and imaginary parts of the magnon eigenfrequencies when $k_x = 0.07\text{nm}^{-1}$. (e-f) With charge current corresponding to $\omega_c = 0.9\kappa$ and magnetic field $H_x = 1.1\times10^5$A/m, the real and imaginary parts of two magnon eigenfrequencies as functions of the wave vector $k_x$. The green points indicate BIC.

which results in magnons possessing a positive imaginary part over an extended range of $k_x$. Consequently, inducing a spin-flop state by the application of magnetic field $H_x$, simplifies the generation of magnon BICs at comparatively lower current densities.

## VIII. BIC WITHIN FERROMAGNETIC COUPLED WAVEGUIDES

The main article employs coupled magnonic waveguides characterized by antiferromagnetic coupling. Here, we explore the possibility of BIC modes in ferromagnetically coupled waveguides, emphasizing the essential role of antiferromagnetic coupling structures. Two

waveguides with ferromagnetic coupling lead to the following magnonic Hamiltonian,

$$\hat{H}_{\mathrm{t}} = \begin{pmatrix} (1-i\alpha)\omega_{\mathrm{f}} - (\alpha\omega_{\mathrm{J1}} + i\omega_{\mathrm{J1}}) & -(1-i\alpha)q \\ -(1-i\alpha)q & (1-i\alpha)\omega_{\mathrm{f}} - (\alpha\omega_{\mathrm{J2}} + i\omega_{\mathrm{J2}}) \end{pmatrix}. \tag{S8}$$

Here, we define $q = \frac{\gamma J_{\mathrm{FM}}}{\mu_0 M_{\mathrm{s}} t}$, $\omega_{\mathrm{f}} = \frac{\gamma}{1+\alpha^2}(H_{\mathrm{a}} + \frac{2A_{\mathrm{ex}}k_{\mathrm{x}}^2}{\mu_0 M_{\mathrm{s}}}) + q$. $J_{\mathrm{FM}}$ is the interlayer ferromagnetic coupling exchange constant, $H_{\mathrm{a}}$ is the applied magnetic field, $\alpha$ is the Gilbert damping constant, $A_{\mathrm{ex}}$ is the intralayer exchange constant, and $k_{\mathrm{x}}$ is the wave vector. The electric current torque term $\omega_{\mathrm{J1,J2}} = \frac{\gamma c_{\mathrm{J1,J2}}}{1+\alpha^2}$ is independently varying in two magnetic layers.

Employing the Hamiltonian approach, we determine two magnon eigenmodes,

$$\omega_{\pm} = (1-i\alpha)[\omega_{\mathrm{f}} - i\frac{(\omega_{\mathrm{J1}} + \omega_{\mathrm{J2}})}{2} \pm \sqrt{q^2 - \frac{(\omega_{\mathrm{J1}} - \omega_{\mathrm{J2}})^2}{4}}]. \tag{S9}$$

When the electric current torque is solely applied to one magnetic layer (say $\omega_{\mathrm{J2}} = 0$), to successfully excite a lossless magnon mode, $\omega_{\mathrm{J1}}$ needs to satisfy this condition,

$$\begin{aligned} &\omega_{\mathrm{J1}} = -(\frac{q^2}{\alpha\omega_{\mathrm{f}}} + \alpha\omega_{\mathrm{f}}), \\ \text{or } &\omega_{\mathrm{J1}} = -\frac{2}{1+\alpha^2}(\alpha\omega_{\mathrm{f}} \pm \alpha\sqrt{q^2 + \alpha^2(q^2 - \omega_{\mathrm{f}}^2)}). \end{aligned} \tag{S10}$$

This equation clearly shows that $\omega_{\mathrm{J1}}$ must be negative (i.e. gain) to effectively induce a lossless mode. This feature is in contrast with the BIC induced by loss, as explored in the main article. The present discussion conclusively identifies the necessity of incorporating antiferromagnetic coupling in waveguide structures for the effective formation of BICs.

## REFERENCES


[1] K. Deng, X. Li, and B. Flebus, Phys. Rev. B **107**, L100402 (2023).

[2] R. A. Duine, V. Errani, and J. S. Harms, Phys. Rev. B **108**, 054428 (2023).

[3] C. W. Hsu, B. Zhen, A. D. Stone, J. D. Joannopoulos, and M. Soljačić, Nat. Rev. Mater. **1**, 16048 (2016).

[4] F. H. Stillinger and D. R. Herrick, Phys. Rev. A **11**, 446 (1975).

[5] Y. Yu, X. Xi, and X. Sun, Light Sci. Appl. **11**, 328 (2022).

[6] Y. Han, C. Meng, H. Pan, J. Qian, Z. Rao, L. Zhu, Y. Gui, C.-M. Hu, and Z. An, Sci. Adv. **9**, eadg4730 (2023).
